# Supplementary material for: The Index of Invariance and its Implications for a Parameterized Least Squares Problem
Source: arXiv:2008.11154 source file (2020-09-01)
Supplement: Supplementary file 1 [file appendixE.tex]

\section{Connection with Block Krylov methods}
\label{app:appC}

\green{LC: TODO}

\begin{corollary}
\label{cor:index-general-tridiagonal-block-decomp}
Let $A \in \Fnn$, $\S$ be a subspace. Define the nested sequence of subspaces $\S_0 \subseteq \dots \subseteq \S_i \subseteq \S_{i+1} \subseteq \dots \subseteq S_k$, as $\S_0 = \S$, $\S_{i+1} = \S_i + A\S_i$ and where $k$ is the first index $i$ where $\Indsimple{A}{S_i} = 0$. Then there exist $V_0$, $V_1$, $\dots$, $V_k$ and $W$ where $\begin{bmatrix} V_0 & \dots & V_k & W\end{bmatrix}$ is unitary, where $\begin{bmatrix} V_0 & \dots & V_j \end{bmatrix}$ spans $S_j$ and such that
\begin{equation}
    A = 
    \begin{bmatrix} V_0^* \\ V_1^* \\ \vdots \\ V_{k-1}^* \\ V_k^* \\ W^* \end{bmatrix}
    \begin{bmatrix}
    T_0 & \times & \times & \times & \times & \times \\
    B_0 & T_1    & \times & \times & \times & \times \\
        & B_1    & T_2    & \times & \times & \times \\
        &        & \ddots & \ddots & \vdots & \vdots \\
        &        &        & B_{k-2} & T_{k-1}& \times \\
        &        &        &        & B_{k-1}& T_k    \\
        &        &        &        &        & \times \\
    \end{bmatrix}
    \begin{bmatrix} V_0 & V_1 & \dots & V_{k-1} & V_k & W \end{bmatrix}
\end{equation}
\end{corollary}

\begin{proof}
Since $\spann(V_0) = \S$, there exist $V'$ and $V''$ such that
\[ \begin{bmatrix} 
        V_0^* \\ V'^* \\ V''^* 
    \end{bmatrix} 
        A 
    \begin{bmatrix} 
        V_0 & V' & V'' 
    \end{bmatrix} 
    = 
    \left[
    \begin{array}{c|c|c} 
        T_0 & P & Q \\ \hline
        B_0 & C & R \\ \hline
        0   & D & E 
    \end{array}
    \right],
\]
We then proceed by induction over
\end{proof}
